# Supplementary material for: Tree exploration in dual-memory model
Source: arXiv:2112.13449 source file (2021-12-26)
Supplement: Supplementary file 1 [file appendix_line.tex]

\section{Missing proofs from Section~\ref{sec:line}}
